# Supplementary material for: Complex Principle Kurtosis Analysis
Source: arXiv:2405.12053 source file (2024-05-20)
Supplement: Supplementary file 1 [file 7-appendix.tex]

\appendix

\section{Appendix}

\noindent\textbf{Intersymbol-interference (ISI):}

The index, which is used in \cite{moreau1994one}, evaluates the performance of estimation of the unmixing matrix. Let $\mathbf{P}=\mathbf{W}\mathbf{A}$, where $\mathbf{W}$ is the estimated unmixing matrix and $\mathbf{A}$ is the mixing matrix (For convenience, suppose both matrices are $L \times L$). The ISI is defined as follows

\begin{equation}
    \mathrm{ISI} = \sum_{i=1}^{L}(\sum_{j=1}^{L}\frac{|\mathbf{P}_{ij}|^2}{\max_k |\mathbf{P}_{ik}|^2} - 1) + \sum_{j=1}^{L}(\sum_{i=1}^{L}\frac{|\mathbf{P}_{ij}|^2}{\max_k |\mathbf{P}_{kj}|^2} - 1) .
\end{equation}

It is obvious that, if the unmixing matrix is well-estimated, $\mathbf{P}$ should be close to the identity matrix, hence ISI should be approaching zero. The smaller the ISI is, the better the performance is.

\noindent\textbf{Average correlation coefficient (ACC)}

The correlation coefficient is a common index in evaluating the similarity between two signals. Although this index is inaccurate in evaluating nonorthogonal signals, it still has guiding significance. The correlation coefficient is defined as follows
\begin{equation}
    \mathrm{CC} = \frac{\mathbf{x}_1 \cdot \mathbf{x}_2}{\lVert \mathbf{x}_1 \rVert \lVert \mathbf{x}_2 \rVert} ,
\end{equation}
where $\lVert \cdot \rVert$ means 2-norm.

The higher the correlation coefficient is, the more similar the two signals are, hence the better algorithms perform. In this experiment, we use the average correlation coefficient to quantify the similarity between source signals and estimated signals. The average correlation coefficient is defined as follows
\begin{equation}
    \mathrm{ACC} = \frac{1}{N}\sum_{i=1}^{N}\mathrm{CC}_i,
\end{equation}
where $N$ is the number of source signals and $\mathrm{CC}_i$ means the correlation coefficient of $i$th source signals.

\noindent\textbf{Signal-distortion-ratio (SDR):}

Numerical separation performances are evaluated by SDR \cite{vincent2007first, sawada2013multichannel}. To calculate SDR, we first decompose the estimated signals as
\begin{equation}
    \hat{\mathbf{y}}_i(t) = \mathbf{y}_i(t) + \mathbf{e}_{i}^{\text{spat}}(t) + \mathbf{e}_{i}^{\text{int}}(t) + \mathbf{e}_{i}^{\text{artif}}(t),
\end{equation}
where $\hat{\mathbf{y}}_i$ is the estimated source signals and $\mathbf{y}_i$ is the true source signals. $\mathbf{e}_{i}^{\text{spat}}$, $\mathbf{e}_{i}^{\text{int}}$ and $\mathbf{e}_{i}^{\text{artif}}$ represents spatial distortion, interferences and artifacts \cite{vincent2007first}. The $i$th signal's $\text{SDR}_i$ can be computed as follows
\begin{equation}
    \text{SDR}_i = 10\log_{10}\frac{\displaystyle\sum_t \mathbf{y}_i(t)^2}{\displaystyle\sum_t[\mathbf{e}_{i}^{\text{spat}}(t) + \mathbf{e}_{i}^{\text{int}}(t) + \mathbf{e}_{i}^{\text{artif}}(t)]^2}.
\end{equation}

SDR evaluates the ratio of useful signals and unrelated signals. The larger the value, the fewer irrelevant components there are.
